# Supplementary material for: Hierarchical Transformer for Task Oriented Dialog Systems
Source: arXiv:2011.08067 source file (2021-05-09)
Supplement: Supplementary file 1 [file appendix.tex]

\appendix

% \section{Conversion of Standard Transformer Encoder into HIER Encoder}

% \paragraph{Self-Attention mask for Utterance Encoder}

% \paragraph{Self-Attention mask for Context Encoder}

% \paragraph{Positional Encoding in Utterance Encoder}

% \paragraph{Positional Encoding in Context Encoder}

% \section{Pseudo-Code for the conversion}
% A pseudo code for converting the algorithm is given in 

% \lstinputlisting[language=Python,float=*,caption=]{pseudo-conversion.py}
\section{Model Architectures}

The model architectures for all model variants are shown below.

\begin{figure}[ht!]
     \centering
     \begin{subfigure}[b]{\linewidth}
        \centering
	    \includegraphics[width=\linewidth]{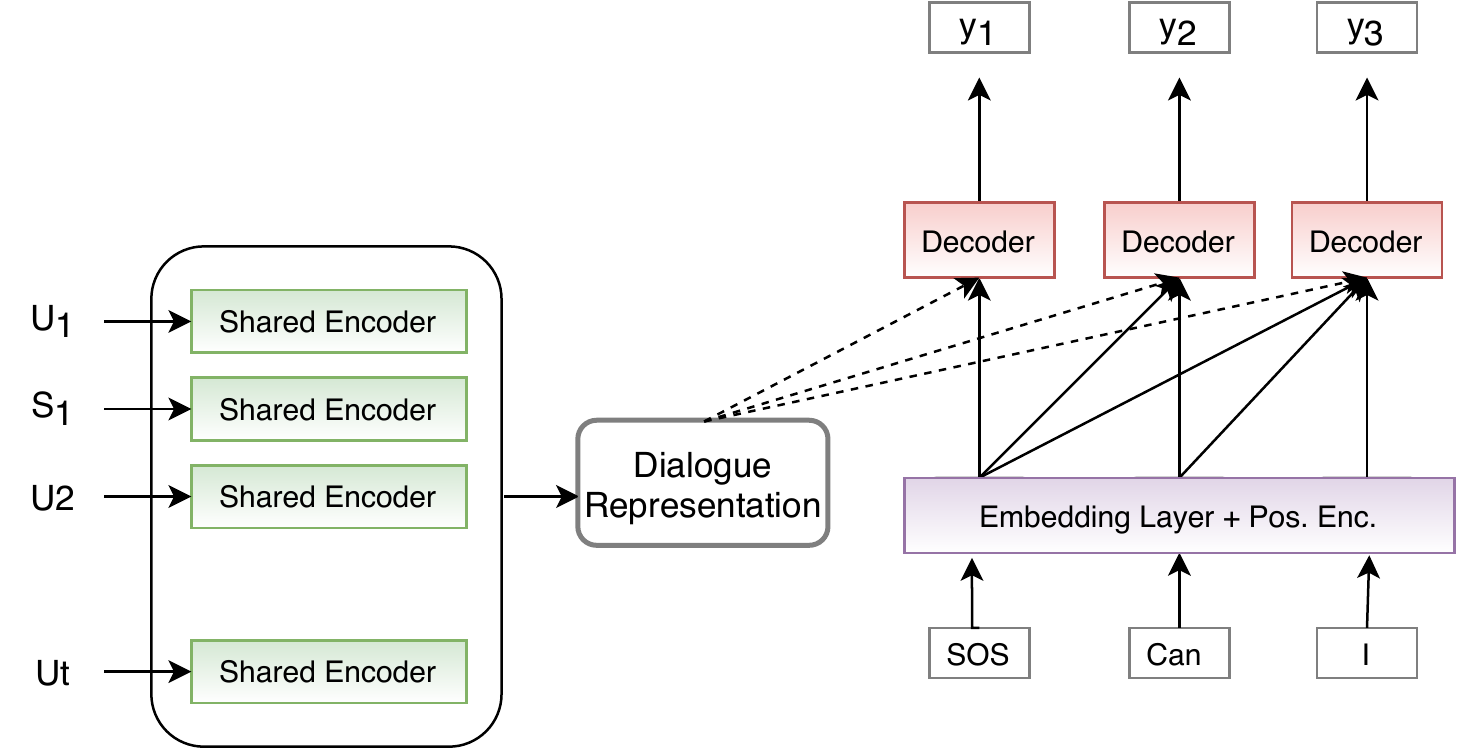}
	    % \includesvg[width=\columnwidth]{figures_svg/baseline.svg}
	    \caption{\textbf{Model: SET} }
	    \label{fig:set}
     \end{subfigure}
     \hfill
     \begin{subfigure}[b]{\linewidth}
         \centering
	    \includegraphics[width=\linewidth]{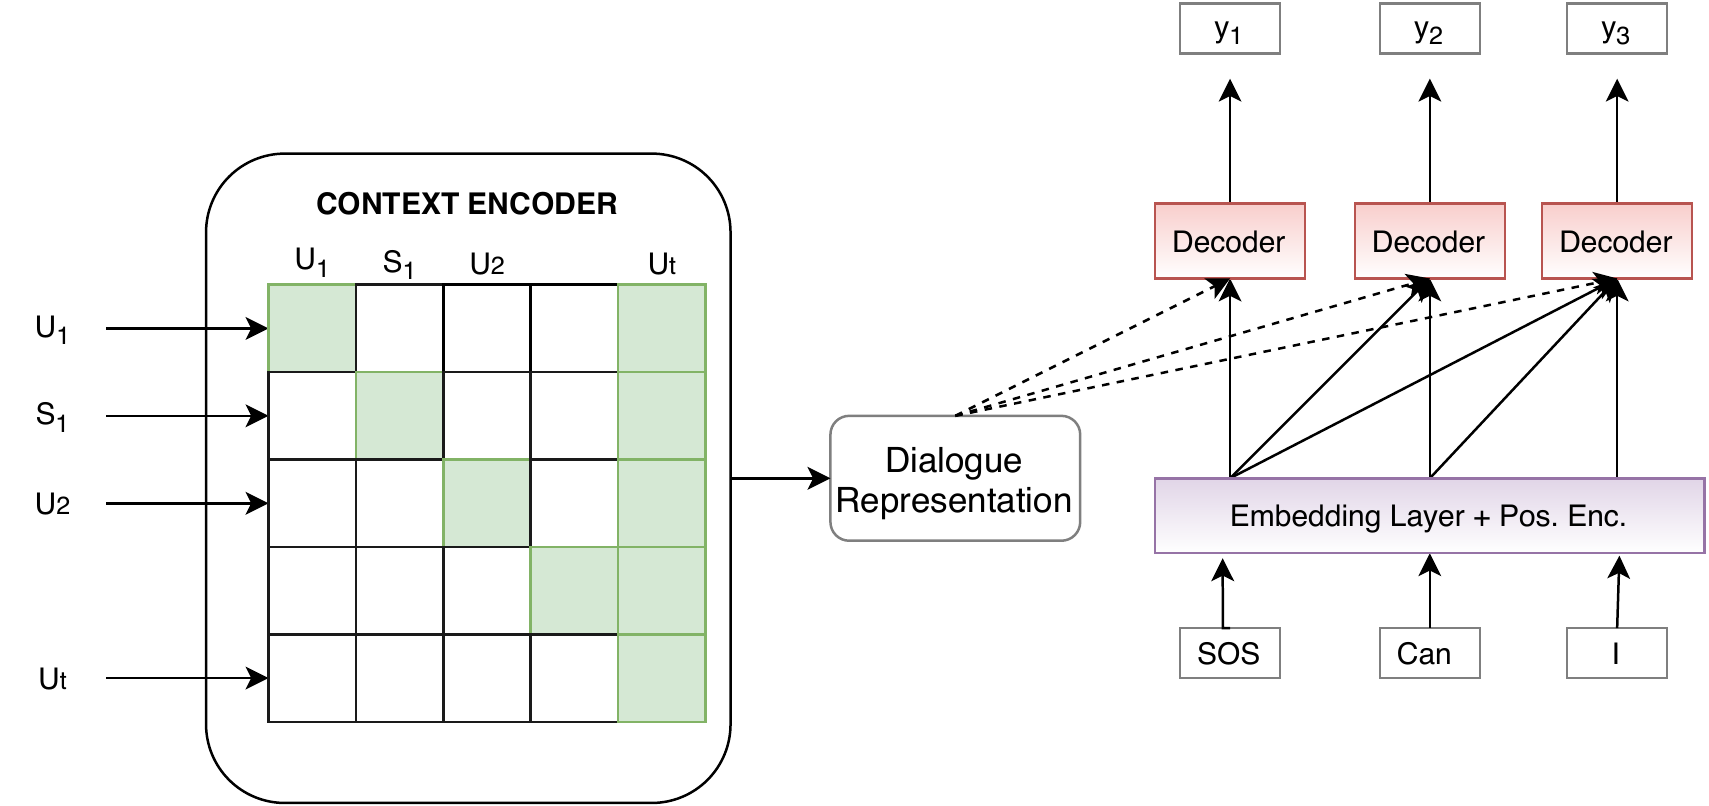}
	     \caption{\textbf{Model: MAT}}
	    \label{fig:mat}
	  \end{subfigure}
	  \hfill
	  \begin{subfigure}[b]{\linewidth}
         \centering
	    \includegraphics[width=\linewidth]{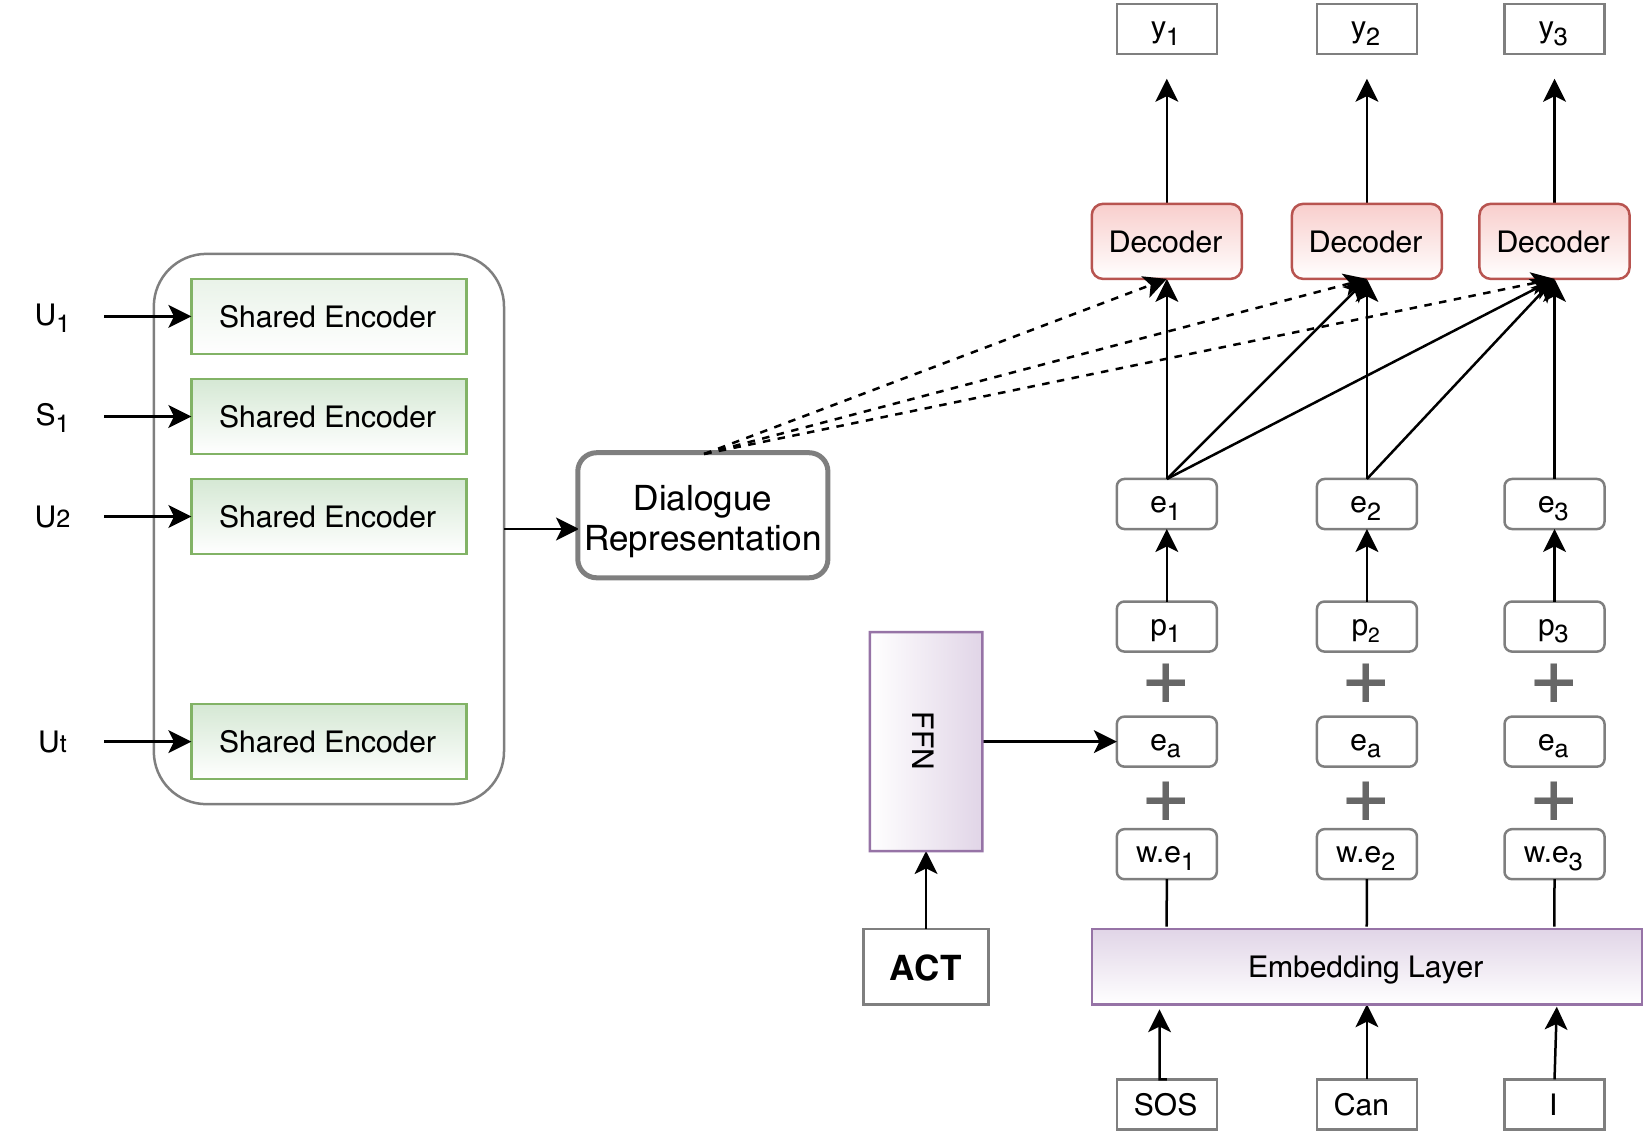}
	     \caption{\textbf{Model: SET++}}
	    \label{fig:my_model3}
     \end{subfigure}
   \caption{Model Variants. Shared Encoder always apply self-attention within utterance bounds. Masked Transformer applies self-attention among all utterances as depicted by the attention mask.}
   \label{fig:models-part1}
\end{figure}

\begin{figure}[ht!]
     \centering
     \begin{subfigure}[b]{\linewidth}
        \centering
	    \includegraphics[width=\linewidth]{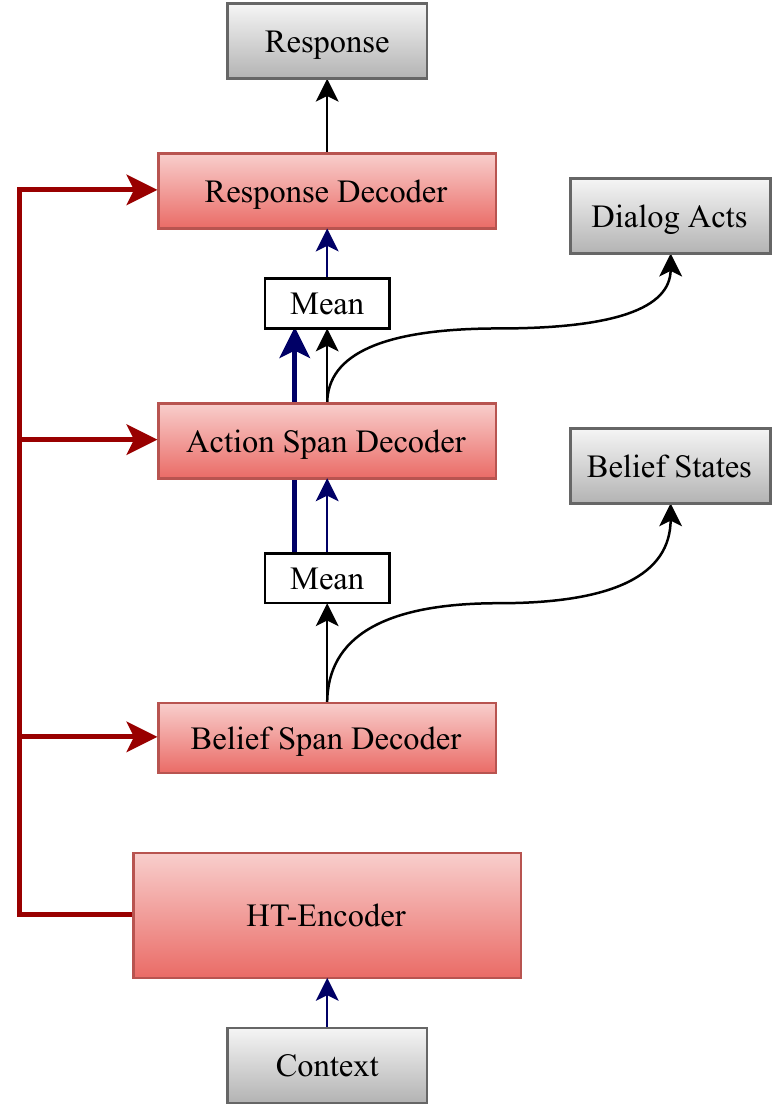}
	    % \includesvg[width=\columnwidth]{figures_svg/baseline.svg}
	    \caption{\textbf{Model: SET} }
	    \label{fig:hier-joint}
     \end{subfigure}
%      \hfill
%      \begin{subfigure}[b]{\linewidth}
%          \centering
% 	    \includegraphics[width=\linewidth]{figures/mat.pdf}
% 	     \caption{\textbf{Model: MAT}}
% 	    \label{fig:mat}
% 	  \end{subfigure}
% 	  \hfill
% 	  \begin{subfigure}[b]{\linewidth}
%          \centering
% 	    \includegraphics[width=\linewidth]{figures/set++.pdf}
% 	     \caption{\textbf{Model: SET++}}
% 	    \label{fig:my_model3}
%      \end{subfigure}
   \caption{Block diagram of the HIER-Joint Architecture. Red links are cross attention from decoder to HT-Encoder. Blue links denote the mean token embeddings from predictions of the previous block.}
   \label{fig:models-part1}
\end{figure}

\section{Hyperparameter Bounds}
Hyperparameter search was executed in the range of parameters as shown below.

\begin{verbatim}
{
    'nhead': [2, 8]
    'embedding_perhead': [25, 40],
    'nhid_perhead': [10, 40],
    'nlayers_e1': [2, 6],
    'nlayers_e2': [2, 6],
    'nlayers_d': [2, 6],
    'dropout': [0.05, 0.8]
}
\end{verbatim}
